# Supplementary material for: Network Representation Learning: Consolidation and Renewed Bearing
Source: arXiv:1905.00987 source file (2019-06-15)
Supplement: Supplementary file 1 [file appendix.tex]

\section{Appendix}

In this section, we report the results on the additional experiments. Specifically, we show the robustness of embedding methods on the link prediction task, the impact of removal of each heuristic feature from both link and node heuristics baseline on the downstream performance. We also report the impact of embedding size and the impact of embedding normalization on downstream machine learning tasks. The node classification performance of embedding methods on 10:90 train:test split is also discussed.

\begin{itemize}

\item \textbf{Impact of embedding dimension:}
We study the impact of embedding size for all the embedding methods on both link prediction and node classification tasks. Specifically, we compare the performances of 64 dimensional embedding with 128 dimensional embedding. The improvement -- quantified in terms of performance difference -- obtained with 128 dimensional embedding over 64 dimensional embedding is reported in Figure \ref{fig:lp_dim} and \ref{fig:nc_dim}. The box-plot represents the distribution of differences in selected performance metric between 128 dimensional embedding and 64 dimensional embedding for each method on all datasets. In link prediction, we observe a statistically significant improvement at significance level 0.05 with the 128 dimensional embedding for Laplacian Eigmaps, GraREP, HOPE, NetMF and MNMF methods. While in node classification, none of the evaluated methods obtained a statistically significant improvement -- at significance level 0.05 --  with 128 embedding dimension. 

%This result strongly suggests that it might be sufficient to obtain a powerful representation with a lower dimensional embedding such as size 64 dimensions rather than conventionally default 128 dimensions, especially for the task of node classification. 

\item \textbf{Impact of embedding normalization on downstream performance:}
We study the impact of L2 normalization the embeddings for both link prediction and node classification tasks. The  comparison results are shown in Figure \ref{fig:lp_l2norm} and Figure \ref{fig:nc_l2norm}. The box plot represents the distribution of differences of AUROC (in Figure \ref{fig:lp_l2norm}) and Micro-f1 scores (in Figure \ref{fig:nc_l2norm}) between normalized and unnormalized embeddings on link prediction and node classification task, respectively. The positive difference implies L2 normalization results in better downstream performance. In link prediction task, %the positive difference in performance between normalized and unnormalized embeddings is statistically significant at significance level 0.1 for VAG while the 
negative difference is statistically significant for VERSE and GraREP at significance level of 0.05 with paired t-test. However, surprisingly the difference in performance with respect to normalization of embeddings is not statistically significantly for rest of the methods for both link prediction. In node classification, the positive difference is  statistically significantly for SDNE and NetMF methods at significance level 0.05 with paired t-test. %NetMF is the only model which highly benefited with the usage of normalization.

%only VAG model obtains statistically significant improvements with p<$0.1$. VERSE, GraREP and WYS obtain a statistically significant negative result with p<$0.1$ on the usage of normalization, which can be seen from the boxplot. 

%The rest of the models do not seem to be significantly impacted by the L2 normalization of embeddings. For the task of node classification, only SDNE and NetMF are significantly (p<$0.5$) impacted with the normalization. NetMF is the only model which highly benefited with the usage of normalization.

\item \textbf{Node classification performance on 10:90 train: test split:} We report the node classification performance of all methods on all the evaluated datasets with 10:90 train:test split in with logistic regression classifier in Figure \ref{fig:node_micro_lr_10} and non-linear classifier EigenPro in Figure \ref{fig:node_micro_eig_10}. The Mean Rank and Mean Penalty of embedding methods – on the datasets for which all methods run to completion on our system – is shown in Figure \ref{fig:mr_op_nc_all_10} . We also report the Mean Rank and Mean Penalty of embedding methods – on datasets with few labels – in Figure \ref{fig:mr_op_nc_10}. The observations we reported in section \ref{nc_results} with train:test 50:50 split also seem to hold with train:test 10:90 split. Specifically, we observe NetMF is the most competitive method for node classification while Laplacian Eigenmaps method outperforms multiple existing methods on multiple datasets (Blogcatalog, Co-author datasets).  Embedding methods such as DeepWalk and LINE also perform well on most datasets.

\end{itemize}

\begin{comment}

\begin{figure}[t]
\centering
\includegraphics[width=0.85\linewidth]{charts/nc_penalty_10.pdf}
  \caption{Mean Rank and Mean Penalty -- on all datasets where all methods finish execution -- for node classification with selected performance metric as Micro-f1 and Logistic Regression classifier.}
  \label{fig:mr_op_nc_all_10}
\end{figure}
%\vspace{-10em}
\begin{figure}
\centering
\includegraphics[width=1.0\linewidth]{charts/nc_penalty_small_10.pdf}
\caption{The Mean Rank and Mean Penalty -- on  datasets with few labels -- for node classification with selected performance metric as Micro-f1 and Logistic Regression classifier.}
\label{fig:mr_op_nc_10}
\end{figure}

\begin{figure}[t]
\centering

\includegraphics[width=0.95\linewidth]{charts/nc_dim_eig.pdf}
  \caption{Impact  of  embedding  dimension on node classification with EigenPro classifier.}
  \label{fig:nc_dim}
\end{figure}
%\vspace{-10em}

\end{comment}
